# Supplementary material for: Electrochemical membrane microactuator with a millisecond response time
Source: arXiv:1801.00481 source file (2018-01-01)
Supplement: Supplementary file 1 [file SM.pdf]

SUPPLEMENTARY MATERIAL

# Electrochemical membrane microactuator with a millisecond response time

Ilia V. Uvarov,[1] Mikhail V. Lokhanin,[2] Alexander V. Postnikov,[1] Artem E. Melenev,[2] and Vitaly B. Svetovoy[3,1,a)]
[1)] *Yaroslavl Branch of the Institute of Physics and Technology RAS, 150007, Universitetskaya 21, Yaroslavl, Russia*
[2)] *P. G. Demidov Yaroslavl State University, Sovetskaya 14, 150000 Yaroslavl, Russia*
[3)] *Zernike Institute for Advanced Materials, University of Groningen - Nijenborgh 4, 9747 AG Groningen, The Netherlands*

## HOMODYNE QUADRATURE INTERFEROMETER

The actuator was characterized by a homemade interferometer that has to be described in some detail. The optical scheme is shown in Fig. S1. The beam of a stabilised He-Ne laser (1) is passed through a polarizing filter (2) and a beam splitter (4). The beam is focused on the membrane (6) by a 10× objective lens (5). A retroreflector (3) allows one to arrange two quadrature signals shifted by a phase. These signals are peaked up by photodetectors (7).

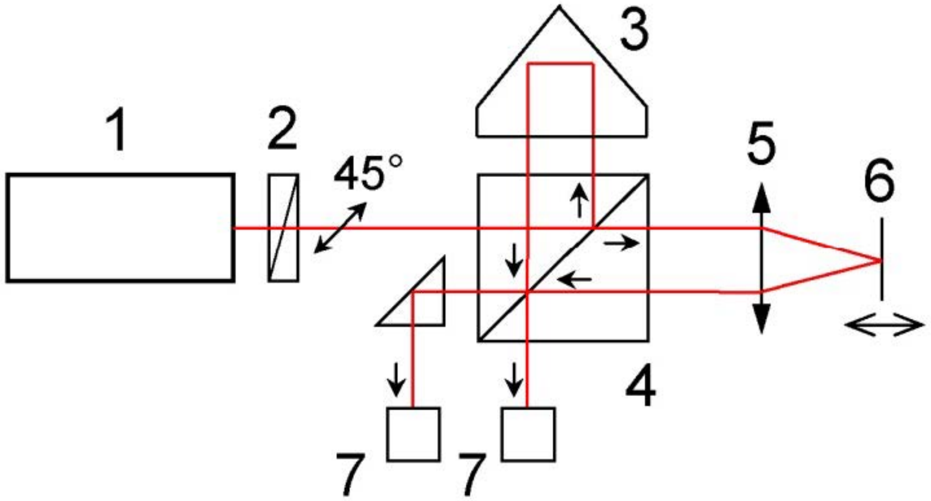


FIG. S1. Optical scheme of the homodyne Michelson interferometer with quadrature signals: (1) stabilized He-Ne laser, (2) polarizing filter, (3) retroreflector, (4) beamsplitter, (5) objective lens, (6) tested sample, (7) photodetectors

The signals registered by each detector can be presented in the form

$$\begin{aligned} I_1(t) &= A_1 + B_1 \cos\varphi(t), \\ I_2(t) &= A_2 + B_2 \cos(\varphi(t)+\varphi_0), \end{aligned} \tag{S1}$$

where the parameters $A_{1,2}$, $B_{1,2}$, and $\varphi_0$ are slowly varying functions of time and the deflection of the membrane can be extracted from the phase $\varphi(t)$ that is given by

$$\varphi(t) = \frac{4\pi d(t)}{\lambda}. \tag{S2}$$

Here $\lambda$ is the laser wavelength and $d(t)$ is the current deflection of the membrane, which we are looking for.

Equations (S1) describe an ellipse in $I_1 - I_2$ plane. Position, axes, and orientation of this ellipse slowly vary with time due to many reasons. If in the limited interval of time these parameters can be considered as constant, then

[a)] Corresponding author: v.b.svetovoy@rug.nl

using the measured signals $I_1(t)$ and $I_2(t)$ we can find the deflection of the membrane $d(t)$. Raw signals for the driving voltage amplitude $U = 11$ V and frequency $f = 500$ kHz are shown in Fig. S2 (left axis) for a series consisting of $N = 40\,000$ pulses.

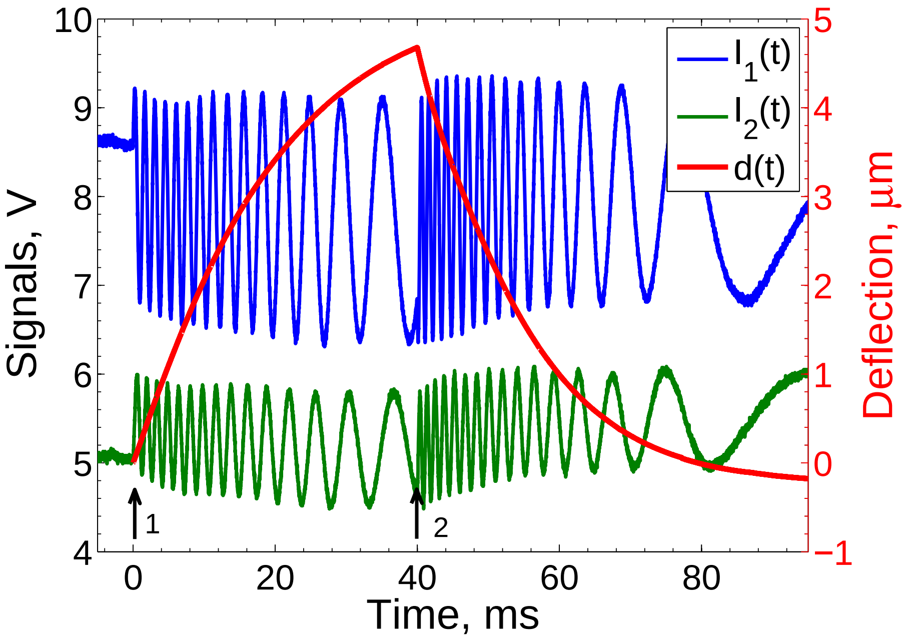


FIG. S2. (left axis) Two phase-shifted raw signals of the interferometer. The electrical pulses are switched on in the moment shown by the arrow 1 and are switched off in the moment shown by the arrow 2. (right axis) The displacement of the membrane restored from the raw signals. When the electrical pulses are switched off the membrane is going down.

One can see that the signals $I_1(t)$ and $I_2(t)$ are looking similar but shifted in a phase. One can get the membrane displacement from each signal separately by counting the fringes, but using both of the signals the deflection can be restored in any moment of time. The red curve in Fig. S2 (right axis) shows the restored deflection. In Fig. S3 the signals are presented in $I_1 - I_2$ plane for the time intervals near the beginning of the series ($0 < t < 1.4$ ms, red points) and near the end of the series ($40 < t < 40.9$ ms, blue points). Only 0.5% of points is shown for readability. One can see that the points lie near a well defined ellipse, but the ellipses near different moments of time are different. This is because the parameters in Eq. (S1) are not constant but slow functions of time.

To find the phase $\varphi(t)$ (or deflection $d(t)$) from the raw signals we are using adaptive time intervals. For each interval the points lie on a half-ellipse and the parameters are determined on this interval from the best fit by the ellipse. However, to take into account small variation of the parameters between two adjacent time intervals, we move between them by smaller steps in time always keep in the buffer the points that form about half of the ellipse. The parameters are refined at each substep so that big jumps in the parameter values are excluded.

## DESCRIPTION OF VIDEOS

**Video S1.** Side view of the membrane recorded at 6000 fps and played at 75 fps. The membrane is driven by a single series of pulses. The process parameters are $U = 14$ V, $f = 500$ kHz, $N = 20\,000$. The maximum deflection of the membrane is estimated as 10.8 $\mu$m.

**Video S2.** Top view of the actuator with the transparent membrane driven by a single series of pulses. The video was recorded at 3 000 fps and it is played at 60 fps. The process parameters are $U = 12$ V, $f = 500$ kHz, $N = 20\,000$. The video demonstrates absence of light scattering objects in the chamber during the process.

**Video S3.** Side view of the membrane demonstrating an explosion in the chamber. The process is driven by a single series of pulses with the parameters: $U = 15$ V, $f = 500$ kHz, $N = 26\,000$. The video was recoded at 10 000 fps and is

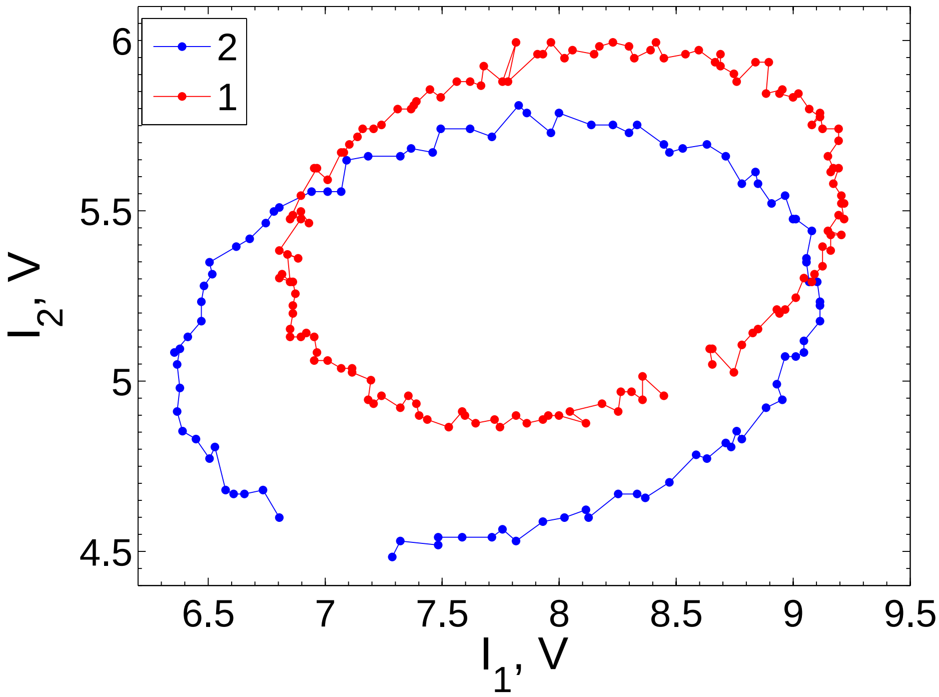


FIG. S3. The raw signals from the interferometer plotted in $I_1 - I_2$ plane. The red dots (1) show the points in the time interval $0 < t < 1.4$ ms. The blue dots (2) present the points in the interval $40 < t < 40.9$ ms immediately after switching off the pulses.

played at 15 fps.

**Video S4.** Side view of the membrane demonstrating cyclic performance of the actuator. The operating frequency is $f_c = 376$ Hz. The video was recorded at 6 000 fps and it is played at 60 fps. The process parameters are: $U = 21$ V, $f = 500$ kHz, $N = 600$.
